# Supplementary material for: Dynamical supersymmetry enhancement of black hole horizons
Source: arXiv:1910.01080 source file (2020-03-27)
Supplement: Supplementary file 2 [file b.tex]

\chapter{}
